# Supplementary material for: van der Waals density functional with corrected $C_6$ coefficients
Source: arXiv:1905.07757 source file (2019-05-19)
Supplement: Supplementary file 1 [file Supplemental_Information.pdf]

# — Supplemental Information —

# A non-local van der Waals density functional with corrected $C_6$ coefficients

K. Berland,[1,2,*] D. Chakraborty,[3,4] and T. Thonhauser[3,4,†]

[1]*Faculty of Science and Technology, Norwegian University of Life Sciences, Norway.*
[2]*Centre for Materials Science and Nanotechnology, University of Oslo, Norway.*
[3]*Department of Physics, Wake Forest University, Winston-Salem, NC 27109, USA.*
[4]*Center for Functional Materials, Wake Forest University, Winston-Salem, NC 27109, USA.*

(Dated: May 13, 2019)

PACS numbers: 71.15.Mb, 31.15.ae, 33.15.Dj

## I. THE NEW KERNEL

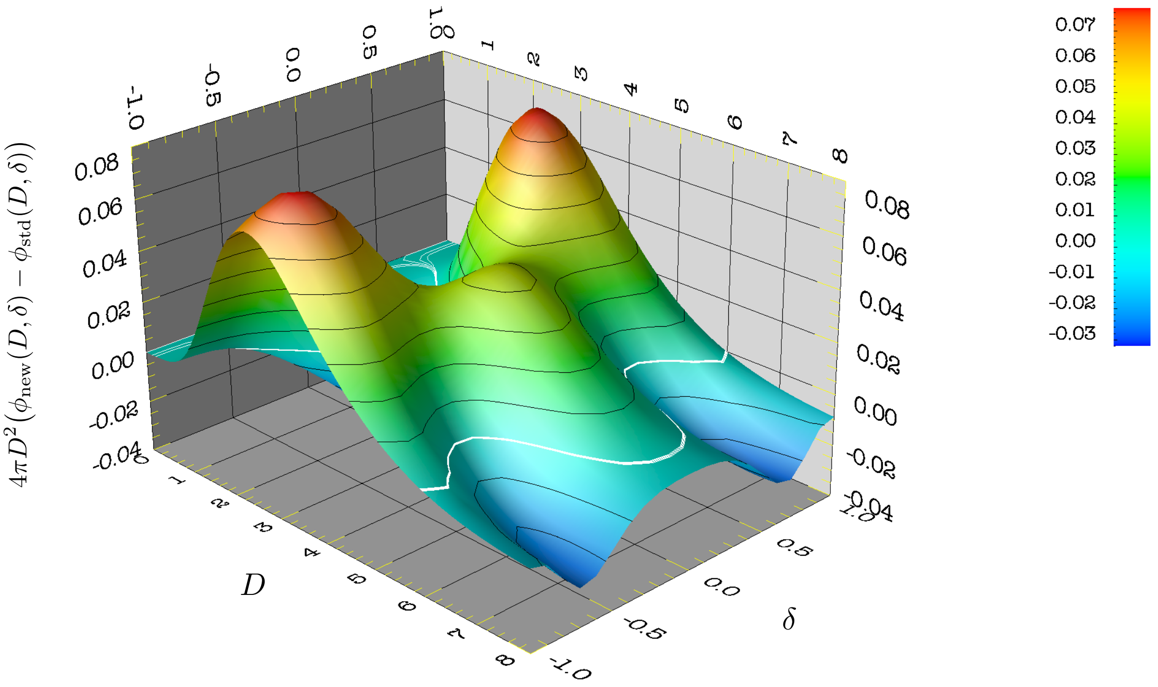


FIG. S1. The difference between our new kernel and the standard kernel, i.e. $4\pi D^2\big(\phi_{\rm new}(D,\delta)-\phi_{\rm std}(D,\delta)\big)$, plotted as a function of $D = (d+d')/2$ and $\delta = (d-d')/(d+d')$, where $0 \le D < \infty$ and $0 \le |\delta| < 1$ and $d = q_0(\mathbf{r})|\mathbf{r}-\mathbf{r}'|$ and $d' = q_0(\mathbf{r}')|\mathbf{r}-\mathbf{r}'|$. Isolines are separated by values of 0.01 and the zero isoline is plotted in white. The standard kernel $\phi_{\rm std}(D,\delta)$ itself is depicted e.g. in Refs. [1 and 2].

## II. BINDING SEPARATION AND BINDING ENERGIES FOR THE S22 DATA SET

TABLE S1. Binding separations [Å] for the S22 set of molecular dimers. The CCSD(T) reference values are taken from Ref. [3].

| No. | Complex (Symmetry) | CCSD(T) | DF1 | DF1-optB88 | DF1-cx | DF2 | DF2-B86R | rVV10 | new |
|---|---|---|---|---|---|---|---|---|---|
| *Hydrogen bonded complexes (7)* | | | | | | | | | |
| 1. | $(NH_3)_2$ ($C_{2h}$) | 3.21 | 3.41 | 3.26 | 3.31 | 3.31 | 3.26 | 3.18 | 3.26 |
| 2. | $(H_2O)_2$ ($C_s$) | 2.91 | 3.03 | 2.93 | 2.93 | 2.98 | 2.91 | 2.88 | 2.91 |
| 3. | Formic acid dimer ($C_{2h}$) | 2.99 | 3.07 | 2.99 | 2.99 | 3.07 | 2.99 | 3.02 | 2.99 |
| 4. | Formamide dimer ($C_{2h}$) | 3.23 | 3.33 | 3.23 | 3.23 | 3.30 | 3.23 | 3.23 | 3.23 |
| 5. | Uracil dimer ($C_{2h}$) | 6.08 | 6.15 | 6.07 | 6.05 | 6.15 | 6.07 | 6.07 | 6.08 |
| 6. | 2-pyridoxine 2-aminopyridine ($C_1$) | 5.14 | 5.21 | 5.11 | 5.11 | 5.21 | 5.11 | 5.14 | 5.11 |
| 7. | Adenine thymine WC complex ($C_1$) | 5.97 | 6.05 | 5.95 | 5.95 | 6.02 | 5.95 | 5.95 | 5.95 |
| | MD [Å] | — | 0.10 | 0.004 | 0.01 | 0.08 | 0.0001 | −0.01 | −0.0001 |
| | MAD [Å] | — | 0.10 | 0.02 | 0.03 | 0.08 | 0.01 | 0.01 | 0.01 |
| | MRD [%] | — | 2.87 | 0.22 | 0.38 | 2.01 | 0.10 | −0.17 | 0.09 |
| | MARD [%] | — | 2.87 | 0.48 | 0.76 | 2.01 | 0.36 | 0.41 | 0.36 |
| *Dispersion dominated complexes (8)* | | | | | | | | | |
| 8. | $(CH_4)_2$ ($D_{3d}$) | 3.72 | 3.89 | 3.82 | 3.97 | 3.69 | 3.82 | 3.67 | 3.84 |
| 9. | $(C_2H_4)_2$ ($D_{2d}$) | 3.72 | 4.07 | 3.87 | 4.17 | 3.87 | 3.89 | 3.74 | 3.89 |
| 10. | Benzene $CH_4$($C_3$) | 3.72 | 4.07 | 3.84 | 4.02 | 3.89 | 3.87 | 3.79 | 3.87 |
| 11. | Benzene dimer ($C_{2h}$) | 3.76 | 4.21 | 3.94 | 4.09 | 4.06 | 3.99 | 3.96 | 3.96 |
| 12. | Pyrazine dimer ($C_s$) | 3.48 | 3.85 | 3.60 | 3.70 | 3.73 | 3.65 | 3.63 | 3.63 |
| 13. | Uracil dimer ($C_2$) | 3.17 | 3.39 | 3.19 | 3.24 | 3.29 | 3.22 | 3.19 | 3.19 |
| 14. | Indole benzene ($C_1$) | 3.50 | 3.90 | 3.65 | 3.75 | 3.80 | 3.70 | 3.67 | 3.67 |
| 15. | Adenine thymine stack ($C_1$) | 3.17 | 3.47 | 3.25 | 3.27 | 3.37 | 3.25 | 3.25 | 3.25 |
| | MD [Å] | — | 0.33 | 0.12 | 0.25 | 0.18 | 0.14 | 0.08 | 0.13 |
| | MAD [Å] | — | 0.33 | 0.12 | 0.25 | 0.19 | 0.14 | 0.10 | 0.13 |
| | MRD [%] | — | 9.28 | 3.22 | 6.83 | 5.25 | 4.01 | 2.39 | 3.73 |
| | MARD [%] | — | 9.28 | 3.22 | 6.83 | 5.42 | 4.01 | 2.73 | 3.73 |
| *Mixed complexes (7)* | | | | | | | | | |
| 16. | Ethene ethyne ($C_{2v}$) | 4.42 | 4.57 | 4.42 | 4.52 | 4.47 | 4.45 | 4.37 | 4.45 |
| 17. | Benzene $H_2O$ ($C_s$) | 3.38 | 3.58 | 3.38 | 3.43 | 3.48 | 3.38 | 3.33 | 3.41 |
| 18. | Benzene $NH_3$ ($C_s$) | 3.56 | 3.84 | 3.61 | 3.74 | 3.69 | 3.64 | 3.56 | 3.63 |
| 19. | Benzene HCN ($C_s$) | 3.95 | 4.20 | 4.00 | 4.03 | 4.10 | 4.00 | 3.98 | 4.00 |
| 20. | Benzene dimer ($C_{2v}$) | 4.91 | 5.23 | 5.03 | 5.11 | 5.13 | 5.06 | 5.01 | 5.03 |
| 21. | Indole benzene T-shape ($C_1$) | 4.88 | 5.16 | 4.98 | 5.03 | 5.08 | 4.98 | 4.96 | 4.98 |
| 22. | Phenol dimer ($C_1$) | 4.92 | 5.12 | 4.95 | 4.97 | 5.02 | 4.95 | 4.92 | 4.95 |
| | MD [Å] | — | 0.24 | 0.05 | 0.11 | 0.14 | 0.06 | 0.01 | 0.06 |
| | MAD [Å] | — | 0.24 | 0.05 | 0.11 | 0.14 | 0.06 | 0.04 | 0.06 |
| | MRD [%] | — | 5.67 | 1.11 | 2.68 | 3.16 | 1.37 | 0.23 | 1.40 |
| | MARD [%] | — | 5.67 | 1.11 | 2.68 | 3.16 | 1.37 | 0.97 | 1.40 |
| *All complexes (22)* | | | | | | | | | |
| | MD [Å] | — | 0.23 | 0.06 | 0.13 | 0.13 | 0.07 | 0.03 | 0.07 |
| | MAD [Å] | — | 0.23 | 0.06 | 0.14 | 0.14 | 0.08 | 0.05 | 0.07 |
| | MRD [%] | — | 6.09 | 1.59 | 3.46 | 3.56 | 1.92 | 0.89 | 1.83 |
| | MARD [%] | — | 6.09 | 1.68 | 3.58 | 3.62 | 2.01 | 1.43 | 1.92 |

TABLE S2. The optimum binding energies [meV] for the S22 set of molecular dimers. The CCSD(T) reference values are taken from Ref. [3].

| No. | Complex (Symmetry) | CCSD(T) | DF1 | DF1-optB88 | DF1-cx | DF2 | DF2-B86R | rVV10 | new |
|---|---|---|---|---|---|---|---|---|---|
| *Hydrogen bonded complexes (7)* | | | | | | | | | |
| 1. | $(NH_3)_2$ ($C_{2h}$) | −137 | −114 | −123 | −115 | −131 | −126 | −147 | −126 |
| 2. | $(H_2O)_2$ ($C_s$) | −218 | −178 | −204 | −192 | −209 | −208 | −237 | −209 |
| 3. | Formic acid dimer ($C_{2h}$) | −815 | −671 | −814 | −793 | −737 | −804 | −858 | −810 |
| 4. | Formamide dimer ($C_{2h}$) | −699 | −569 | −670 | −641 | −629 | −659 | −714 | −666 |
| 5. | Uracil dimer ($C_{2h}$) | −897 | −748 | −863 | −836 | −806 | −846 | −900 | −863 |
| 6. | 2-pyridoxine 2-aminopyridine ($C_1$) | −737 | −627 | −741 | −724 | −669 | −722 | −774 | −741 |
| 7. | Adenine thymine WC complex ($C_1$) | −726 | −598 | −712 | −686 | −643 | −689 | −750 | −712 |
| | MD [meV] | — | 103 | 14.7 | 34.9 | 58.0 | 25.1 | −21.4 | 14.9 |
| | MAD [meV] | — | 103 | 15.7 | 34.9 | 58.0 | 25.1 | 21.4 | 15.9 |
| | MRD [%] | — | −17.2 | −3.75 | −7.67 | −8.50 | −4.72 | 4.50 | −3.30 |
| | MARD [%] | — | 17.2 | 3.88 | 7.67 | 8.50 | 4.72 | 4.50 | 3.43 |
| *Dispersion dominated complexes (8)* | | | | | | | | | |
| 8. | $(CH_4)_2$ ($D_{3d}$) | −23.0 | −37.0 | −24.3 | −31.8 | −30.8 | −20.6 | −21.2 | −23.0 |
| 9. | $(C_2H_4)_2$ ($D_{2d}$) | −65.0 | −64.9 | −57.1 | −57.8 | −64.2 | −49.7 | −59.9 | −54.0 |
| 10. | Benzene $CH_4$($C_3$) | −62.9 | −67.4 | −66.9 | −62.6 | −63.4 | −53.5 | −62.1 | −62.2 |
| 11. | Benzene dimer ($C_{2h}$) | −114 | −136 | −150 | −129 | −125 | −107 | −125 | −137 |
| 12. | Pyrazine dimer ($C_s$) | −182 | −183 | −206 | −180 | −176 | −162 | −179 | −192 |
| 13. | Uracil dimer ($C_2$) | −422 | −395 | −453 | −404 | −393 | −383 | −409 | −435 |
| 14. | Indole benzene ($C_1$) | −199 | −205 | −239 | −202 | −198 | −181 | −205 | −225 |
| 15. | Adenine thymine stack ($C_1$) | −506 | −454 | −540 | −474 | −458 | −453 | −488 | −523 |
| | MD [meV] | — | 3.98 | −20.4 | 3.95 | 8.17 | 20.5 | 2.98 | −9.76 |
| | MAD [meV] | — | 15.8 | 22.4 | 10.9 | 13.0 | 20.5 | 7.28 | 12.7 |
| | MRD [%] | — | 9.26 | 9.95 | 3.82 | 2.88 | −11.9 | −1.54 | 3.43 |
| | MARD [%] | — | 13.5 | 13.0 | 9.66 | 8.26 | 11.9 | 4.73 | 7.98 |
| *Mixed complexes (7)* | | | | | | | | | |
| 16. | Ethene ethyne ($C_{2v}$) | −65.5 | −68.3 | −67.3 | −65.7 | −68.3 | −62.5 | −71.6 | −65.5 |
| 17. | Benzene $H_2O$ ($C_s$) | −143 | −121 | −136 | −126 | −125 | −124 | −142 | −131 |
| 18. | Benzene $NH_3$ ($C_s$) | −101 | −93.0 | −98.0 | −91.6 | −91.8 | −85.5 | −97.1 | −93.7 |
| 19. | Benzene HCN ($C_s$) | −197 | −162 | −184 | −175 | −164 | −172 | −181 | −179 |
| 20. | Benzene dimer ($C_{2v}$) | −118 | −114 | −123 | −114 | −105 | −97.4 | −110 | −116 |
| 21. | Indole benzene T-shape ($C_1$) | −244 | −212 | −239 | −226 | −202 | −207 | −227 | −232 |
| 22. | Phenol dimer ($C_1$) | −307 | −249 | −295 | −262 | −270 | −263 | −300 | −285 |
| | MD [meV] | — | 22.2 | 4.74 | 16.4 | 21.1 | 23.3 | 6.53 | 10.4 |
| | MAD [meV] | — | 23.0 | 6.70 | 16.5 | 21.9 | 23.3 | 8.29 | 10.4 |
| | MRD [%] | — | −10.2 | −1.88 | −8.16 | −10.4 | −13.2 | −2.63 | −5.40 |
| | MARD [%] | — | 11.4 | 3.89 | 8.24 | 11.7 | 13.2 | 5.31 | 5.42 |
| *All complexes (22)* | | | | | | | | | |
| | MD [meV] | — | 41.4 | −1.24 | 17.8 | 28.2 | 22.9 | −3.64 | 4.49 |
| | MAD [meV] | — | 46.0 | 15.3 | 20.3 | 30.2 | 22.9 | 12.1 | 13.0 |
| | MRD [%] | — | −5.35 | 1.83 | −3.65 | −4.97 | −10.0 | 0.04 | −1.52 |
| | MARD [%] | — | 14.0 | 7.19 | 8.58 | 9.42 | 10.0 | 4.84 | 5.72 |

## III. BINDING SEPARATION AND BINDING ENERGIES FOR THE S66 DATA SET

TABLE S3. Binding separations [Å] for the S66 data set. CCSD(T)/CBS reference values are taken from Ref. [4]. The following interaction types are mentioned in parenthesis: E = electrostatics-dominated, D = dispersion-dominated, and M = mixed.

| No. | System (interaction type) | CCSD(T)/CBS | DF1 | DF1-optB88 | DF1-cx | DF2 | DF2-B86R | rVV10 | new |
|---|---|---|---|---|---|---|---|---|---|
| *Hydrogen bonded complexes (23)* | | | | | | | | | |
| 1. | Water ··· Water (E) | 1.96 | 2.08 | 1.96 | 1.97 | 2.02 | 1.96 | 1.93 | 1.96 |
| 2. | Water ··· MeOH(E) | 1.92 | 2.03 | 1.92 | 1.93 | 1.97 | 1.91 | 1.90 | 1.92 |
| 3. | Water ··· $MeNH_2$(E) | 1.96 | 2.03 | 1.94 | 1.93 | 2.01 | 1.93 | 1.93 | 1.94 |
| 4. | Water ··· Peptide (E) | 1.86 | 1.97 | 1.86 | 1.87 | 1.92 | 1.86 | 1.85 | 1.86 |
| 5. | MeOH ··· MeOH (E) | 1.91 | 2.02 | 1.90 | 1.91 | 1.97 | 1.90 | 1.89 | 1.90 |
| 6. | MeOH ··· $MeNH_2$ (E) | 1.94 | 2.03 | 1.93 | 1.92 | 2.00 | 1.92 | 1.92 | 1.92 |
| 7. | MeOH ··· Peptide (E) | 1.86 | 1.95 | 1.85 | 1.85 | 1.91 | 1.85 | 1.85 | 1.85 |
| 8. | MeOH ··· Water (E) | 1.95 | 2.07 | 1.95 | 1.96 | 2.01 | 1.95 | 1.92 | 1.95 |
| 9. | $MeNH_2$ ··· MeOH (M) | 2.20 | 2.36 | 2.22 | 2.29 | 2.25 | 2.22 | 2.17 | 2.23 |
| 10. | $MeNH_2$ ··· $MeNH_2$ (M) | 2.24 | 2.42 | 2.26 | 2.30 | 2.33 | 2.26 | 2.23 | 2.27 |
| 11. | $MeNH_2$ ··· Peptide (M) | 2.20 | 2.37 | 2.23 | 2.26 | 2.29 | 2.23 | 2.21 | 2.24 |
| 12. | $MeNH_2$ ··· Water (E) | 1.94 | 2.03 | 1.93 | 1.92 | 2.00 | 1.92 | 1.92 | 1.93 |
| 13. | Peptide ··· MeOH (E) | 1.99 | 2.15 | 2.01 | 2.04 | 2.07 | 2.01 | 1.98 | 2.01 |
| 14. | Peptide ··· $MeNH_2$ (E) | 2.05 | 2.17 | 2.04 | 2.05 | 2.13 | 2.04 | 2.04 | 2.05 |
| 15. | Peptide ··· Peptide(E) | 1.95 | 2.08 | 1.96 | 1.97 | 2.02 | 1.96 | 1.94 | 1.96 |
| 16. | Peptide ··· Water (E) | 2.05 | 2.20 | 2.08 | 2.11 | 2.12 | 2.08 | 2.03 | 2.08 |
| 17. | Uracil ··· Uracil (BP) (E) | 1.77 | 1.85 | 1.76 | 1.75 | 1.84 | 1.76 | 1.76 | 1.76 |
| 18. | Water ··· Pyridine (E) | 1.95 | 2.02 | 1.93 | 1.92 | 1.99 | 1.92 | 1.92 | 1.93 |
| 19. | MeOH ··· Pyridine (E) | 1.93 | 2.00 | 1.91 | 1.90 | 1.98 | 1.90 | 1.90 | 1.90 |
| 20. | AcOH ··· AcOH (E) | 1.68 | 1.75 | 1.67 | 1.65 | 1.75 | 1.67 | 1.68 | 1.67 |
| 21. | $AcNH_2$ ··· $AcNH_2$ (E) | 1.84 | 1.93 | 1.84 | 1.83 | 1.91 | 1.84 | 1.84 | 1.84 |
| 22. | AcOH ··· Uracil (E) | 1.70 | 1.77 | 1.69 | 1.67 | 1.76 | 1.68 | 1.69 | 1.68 |
| 23. | $AcNH_2$ ··· Uracil (E) | 1.73 | 1.82 | 1.73 | 1.72 | 1.80 | 1.72 | 1.73 | 1.73 |
| | MD [Å] | — | 0.11 | −0.001 | 0.01 | 0.06 | −0.003 | −0.02 | −0.001 |
| | MAD [Å] | — | 0.11 | 0.01 | 0.03 | 0.06 | 0.01 | 0.02 | 0.01 |
| | MRD [%] | — | 5.55 | −0.08 | 0.20 | 3.26 | −0.19 | −0.80 | −0.07 |
| | MARD [%] | — | 5.55 | 0.54 | 1.32 | 3.26 | 0.72 | 0.80 | 0.68 |
| *Dispersion dominated complexes (23)* | | | | | | | | | |
| 24. | Benzene ··· Benzene ($\pi$–$\pi$) (D) | 3.51 | 3.62 | 3.38 | 3.51 | 3.50 | 3.44 | 3.39 | 3.42 |
| 25. | Pyridine ··· Pyridine ($\pi$–$\pi$) (D) | 3.36 | 3.47 | 3.24 | 3.33 | 3.36 | 3.28 | 3.25 | 3.27 |
| 26. | Uracil ··· Uracil ($\pi$–$\pi$) (M) | 2.69 | 2.93 | 2.73 | 2.79 | 2.83 | 2.75 | 2.74 | 2.74 |
| 27. | Benzene ··· Pyridine ($\pi$–$\pi$) (D) | 3.39 | 3.50 | 3.26 | 3.37 | 3.38 | 3.31 | 3.27 | 3.29 |
| 28. | Benzene ··· Uracil ($\pi$–$\pi$) (D) | 3.10 | 3.38 | 3.15 | 3.22 | 3.27 | 3.18 | 3.16 | 3.17 |
| 29. | Pyridine ··· Uracil ($\pi$–$\pi$) (M) | 3.17 | 3.43 | 3.22 | 3.29 | 3.33 | 3.25 | 3.23 | 3.24 |
| 30. | Benzene ··· Ethene (D) | 3.54 | 3.87 | 3.59 | 3.80 | 3.71 | 3.66 | 3.57 | 3.65 |
| 31. | Uracil ··· Ethene (D) | 2.94 | 3.23 | 3.01 | 3.13 | 3.10 | 3.04 | 2.99 | 3.04 |
| 32. | Uracil ··· Ethyne (M) | 2.91 | 3.17 | 2.96 | 3.05 | 3.04 | 2.99 | 2.94 | 2.99 |
| 33. | Pyridine ··· Ethene (D) | 3.25 | 3.57 | 3.30 | 3.47 | 3.41 | 3.35 | 3.28 | 3.35 |
| 34. | Pentane ··· Pentane (D) | 2.47 | 2.77 | 2.53 | 2.81 | 2.58 | 2.57 | 2.47 | 2.56 |
| 35. | Neopentane ··· Pentane (D) | 2.46 | 2.72 | 2.49 | 2.75 | 2.54 | 2.54 | 2.43 | 2.53 |
| 36. | Neopentane ··· Neopentane (D) | 2.53 | 2.75 | 2.53 | 2.80 | 2.56 | 2.60 | 2.45 | 2.57 |
| 37. | Cyclopentane ··· Neopentane (D) | 2.40 | 2.68 | 2.44 | 2.70 | 2.49 | 2.49 | 2.38 | 2.47 |
| 38. | Cyclopentane ··· Cyclopentane (D) | 2.42 | 2.69 | 2.46 | 2.72 | 2.51 | 2.50 | 2.40 | 2.49 |
| 39. | Benzene ··· Cyclopentane (D) | 2.84 | 3.12 | 2.89 | 3.03 | 2.98 | 2.93 | 2.88 | 2.92 |
| 40. | Benzene ··· Neopentane (D) | 2.94 | 3.22 | 2.99 | 3.14 | 3.08 | 3.04 | 2.96 | 3.02 |
| 41. | Uracil ··· Pentane (D) | 2.82 | 3.11 | 2.88 | 3.06 | 2.96 | 2.92 | 2.86 | 2.91 |
| 42. | Uracil ··· Cyclopentane (D) | 2.70 | 2.99 | 2.76 | 2.95 | 2.84 | 2.80 | 2.73 | 2.78 |
| 43. | Uracil ··· Neopentane (D) | 2.72 | 2.98 | 2.77 | 2.94 | 2.84 | 2.81 | 2.75 | 2.80 |
| 44. | Ethene ··· Pentane (D) | 2.50 | 2.81 | 2.58 | 2.87 | 2.61 | 2.62 | 2.49 | 2.62 |
| 45. | Ethyne ··· Pentane (D) | 2.99 | 3.25 | 3.05 | 3.27 | 3.08 | 3.09 | 2.99 | 3.09 |
| 46. | Peptide ··· Pentane (D) | 2.41 | 2.71 | 2.48 | 2.71 | 2.54 | 2.52 | 2.44 | 2.51 |
| | MD [Å] | — | 0.26 | 0.03 | 0.20 | 0.11 | 0.07 | 0.0001 | 0.06 |
| | MAD [Å] | — | 0.26 | 0.06 | 0.21 | 0.11 | 0.09 | 0.04 | 0.08 |
| | MRD [%] | — | 9.25 | 1.15 | 7.55 | 3.87 | 2.60 | 0.04 | 2.28 |
| | MARD [%] | — | 9.25 | 2.11 | 7.65 | 3.90 | 3.18 | 1.46 | 2.98 |

TABLE S3. CONTINUED.

| No. | System (interaction type) | CCSD(T)/CBS | DF1 | DF1-optB88 | DF1-cx | DF2 | DF2-B86R | rVV10 | new |
|---|---|---|---|---|---|---|---|---|---|
| *Others (20)* | | | | | | | | | |
| 47. | Benzene ··· Benzene (TS) (D) | 2.84 | 3.13 | 2.92 | 3.04 | 3.01 | 2.95 | 2.89 | 2.94 |
| 48. | Pyridine ··· Pyridine (TS) (D) | 2.65 | 2.94 | 2.72 | 2.85 | 2.80 | 2.75 | 2.69 | 2.74 |
| 49. | Benzene ··· Pyridine (TS) (D) | 2.82 | 3.10 | 2.89 | 2.99 | 2.98 | 2.92 | 2.87 | 2.91 |
| 50. | Benzene ··· Ethyne (CH ··· $\pi$) (M) | 2.83 | 3.09 | 2.89 | 2.98 | 2.97 | 2.90 | 2.85 | 2.91 |
| 51. | Ethyne ··· Ethyne (TS) (M) | 2.76 | 2.94 | 2.79 | 2.89 | 2.81 | 2.80 | 2.71 | 2.80 |
| 52. | Benzene ··· AcOH (OH ··· $\pi$) (M) | 2.45 | 2.67 | 2.47 | 2.50 | 2.60 | 2.49 | 2.47 | 2.49 |
| 53. | Benzene ··· $AcNH_2$ (NH ··· $\pi$) (M) | 2.55 | 2.78 | 2.59 | 2.65 | 2.68 | 2.60 | 2.56 | 2.60 |
| 54. | Benzene ··· Water (OH ··· $\pi$) (M) | 2.56 | 2.80 | 2.59 | 2.66 | 2.69 | 2.61 | 2.56 | 2.61 |
| 55. | Benzene ··· MeOH (OH ··· $\pi$) (M) | 2.53 | 2.77 | 2.56 | 2.62 | 2.67 | 2.58 | 2.54 | 2.58 |
| 56. | Benzene ··· $MeNH_2$ (NH ··· $\pi$) (D) | 2.72 | 2.99 | 2.78 | 2.88 | 2.87 | 2.80 | 2.76 | 2.80 |
| 57. | Benzene ··· Peptide (NH ··· $\pi$) (M) | 2.65 | 2.90 | 2.70 | 2.77 | 2.80 | 2.72 | 2.69 | 2.72 |
| 58. | Pyridine ··· Pyridine (CH ··· N) (M) | 2.39 | 2.57 | 2.41 | 2.47 | 2.46 | 2.42 | 2.36 | 2.42 |
| 59. | Ethyne ··· Water (CH ··· O) (E) | 2.21 | 2.36 | 2.23 | 2.30 | 2.25 | 2.23 | 2.16 | 2.23 |
| 60. | Ethyne ··· AcOH (OH ··· $\pi$) (E) | 2.28 | 2.44 | 2.28 | 2.29 | 2.37 | 2.28 | 2.25 | 2.28 |
| 61. | Pentane ··· AcOH (D) | 2.34 | 2.70 | 2.50 | 2.72 | 2.55 | 2.54 | 2.46 | 2.53 |
| 62. | Pentane ··· $AcNH_2$ (D) | 2.36 | 2.66 | 2.42 | 2.66 | 2.48 | 2.46 | 2.37 | 2.45 |
| 63. | Benzene ··· AcOH(D) | 2.85 | 3.12 | 2.91 | 3.01 | 3.00 | 2.94 | 2.90 | 2.94 |
| 64. | Peptide ··· Ethene (M) | 2.52 | 2.76 | 2.58 | 2.74 | 2.62 | 2.60 | 2.53 | 2.60 |
| 65. | Pyridine ··· Ethyne (E) | 2.24 | 2.33 | 2.20 | 2.22 | 2.27 | 2.21 | 2.18 | 2.21 |
| 66. | $MeNH_2$ ··· Pyridine (M) | 2.34 | 2.59 | 2.37 | 2.45 | 2.45 | 2.38 | 2.33 | 2.38 |
| | MD [Å] | — | 0.24 | 0.05 | 0.14 | 0.12 | 0.07 | 0.01 | 0.06 |
| | MAD [Å] | — | 0.24 | 0.05 | 0.14 | 0.12 | 0.07 | 0.03 | 0.07 |
| | MRD [%] | — | 9.34 | 1.80 | 5.50 | 4.81 | 2.53 | 0.47 | 2.51 |
| | MARD [%] | — | 9.34 | 1.94 | 5.59 | 4.81 | 2.65 | 1.36 | 2.62 |
| *All complexes (66)* | | | | | | | | | |
| | MD [Å] | — | 0.20 | 0.02 | 0.12 | 0.10 | 0.04 | −0.001 | 0.04 |
| | MAD [Å] | — | 0.20 | 0.04 | 0.12 | 0.10 | 0.06 | 0.03 | 0.05 |
| | MRD [%] | — | 7.99 | 0.92 | 4.37 | 3.94 | 1.61 | −0.12 | 1.53 |
| | MARD [%] | — | 7.99 | 1.52 | 4.82 | 3.96 | 2.16 | 1.20 | 2.07 |

TABLE S4. Binding energies [meV] for the S66 set of molecular dimers. CCSD(T)/CBS reference values are taken from Ref. [4]. The following interaction types are mentioned in parenthesis: E = electrostatics-dominated, D = dispersion-dominated, and M = mixed. The outliers in Fig. 5 in the main manuscript are indicated in red.

| No. | System (interaction type) | CCSD(T)/CBS | DF1 | DF1-optB88 | DF1-cx | DF2 | DF2-B86R | rVV10 | new |
|---|---|---|---|---|---|---|---|---|---|
| *Hydrogen bonded complexes (23)* | | | | | | | | | |
| 1. | Water ··· Water (E) | −213 | −178 | −203 | −190 | −208 | −207 | −234 | −207 |
| 2. | Water ··· MeOH(E) | −242 | −206 | −236 | −222 | −236 | −236 | −260 | −238 |
| 3. | Water ··· $MeNH_2$(E) | −300 | −268 | −312 | −304 | −298 | −314 | −344 | −315 |
| 4. | Water ··· Peptide (E) | −351 | −295 | −342 | −321 | −333 | −337 | −369 | −341 |
| 5. | MeOH ··· MeOH (E) | −250 | −220 | −251 | −238 | −243 | −245 | −266 | −250 |
| 6. | MeOH ··· $MeNH_2$ (E) | −328 | −300 | −346 | −340 | −323 | −342 | −366 | −347 |
| 7. | MeOH ··· Peptide (E) | −357 | −310 | −363 | −344 | −342 | −351 | −382 | −359 |
| 8. | MeOH ··· Water (E) | −217 | −187 | −212 | −202 | −212 | −213 | −237 | −215 |
| 9. | $MeNH_2$ ··· MeOH (M) | −133 | −130 | −136 | −128 | −138 | −127 | −143 | −134 |
| 10. | $MeNH_2$ ··· $MeNH_2$ (M) | −180 | −160 | −181 | −166 | −177 | −173 | −195 | −179 |
| 11. | $MeNH_2$ ··· Peptide (M) | −235 | −206 | −236 | −212 | −224 | −217 | −242 | −228 |
| 12. | $MeNH_2$ ··· Water (E) | −315 | −278 | −324 | −314 | −309 | −325 | −351 | −326 |
| 13. | Peptide ··· MeOH (E) | −268 | −234 | −260 | −242 | −252 | −246 | −269 | −256 |
| 14. | Peptide ··· $MeNH_2$ (E) | −323 | −291 | −333 | −321 | −308 | −318 | −344 | −329 |
| 15. | Peptide ··· Peptide(E) | −374 | −330 | −374 | −351 | −349 | −348 | −380 | −365 |
| 16. | Peptide ··· Water (E) | −222 | −193 | −209 | −197 | −210 | −204 | −227 | −210 |
| 17. | Uracil ··· Uracil (BP) (E) | −745 | −638 | −745 | −718 | −692 | −727 | −782 | −745 |
| 18. | Water ··· Pyridine (E) | −297 | −270 | −310 | −300 | −300 | −309 | −338 | −313 |
| 19. | MeOH ··· Pyridine (E) | −321 | −299 | −343 | −335 | −321 | −335 | −360 | −343 |
| 20. | AcOH ··· AcOH (E) | −828 | −699 | −845 | −826 | −763 | −835 | −890 | −844 |
| 21. | $AcNH_2$ ··· $AcNH_2$ (E) | −705 | −586 | −689 | −661 | −645 | −677 | −733 | −687 |
| 22. | AcOH ··· Uracil (E) | −845 | −717 | −846 | −822 | −780 | −833 | −888 | −846 |
| 23. | $AcNH_2$ ··· Uracil (E) | −832 | −707 | −819 | −792 | −764 | −805 | −857 | −818 |
| | MD [meV] | — | 51.4 | −1.47 | 14.6 | 19.9 | 6.92 | −25.0 | −0.45 |
| | MAD [meV] | — | 51.4 | 8.50 | 17.4 | 20.6 | 13.1 | 25.0 | 9.11 |
| | MRD [%] | — | −12.4 | 0.39 | −4.34 | −3.81 | −2.00 | 7.06 | 0.10 |
| | MARD [%] | — | 12.4 | 2.58 | 5.22 | 4.25 | 3.85 | 7.06 | 2.69 |
| *Dispersion dominated complexes (23)* | | | | | | | | | |
| 24. | Benzene ··· Benzene (π–π) (D) | −122 | −136 | −150 | −129 | −125 | −106 | −124 | −137 |
| 25. | Pyridine ··· Pyridine (π–π) (D) | −169 | −170 | −191 | −167 | −160 | −146 | −163 | −177 |
| 26. | Uracil ··· Uracil (π–π) (M) | −426 | −397 | −454 | −406 | −394 | −385 | −411 | −437 |
| 27. | Benzene ··· Pyridine (π–π) (D) | −149 | −155 | −174 | −151 | −145 | −129 | −147 | −160 |
| 28. | Benzene ··· Uracil (π–π) (D) | −248 | −230 | −267 | −231 | −224 | −210 | −234 | −251 |
| 29. | Pyridine ··· Uracil (π–π) (M) | −296 | −276 | −313 | −275 | −273 | −256 | −280 | −297 |
| 30. | Benzene ··· Ethene (D) | −62.1 | −74.6 | −78.8 | −65.7 | −71.4 | −54.1 | −69.7 | −68.8 |
| 31. | Uracil ··· Ethene (D) | −147 | −144 | −156 | −137 | −143 | −126 | −143 | −144 |
| 32. | Uracil ··· Ethyne (M) | −162 | −156 | −170 | −151 | −161 | −144 | −160 | −160 |
| 33. | Pyridine ··· Ethene (D) | −81.2 | −88.6 | −95.5 | −80.8 | −87.0 | −70.6 | −86.6 | −85.2 |
| 34. | Pentane ··· Pentane (D) | −164 | −191 | −200 | −172 | −186 | −151 | −177 | −180 |
| 35. | Neopentane ··· Pentane (D) | −113 | −137 | −142 | −123 | −130 | −104 | −130 | −127 |
| 36. | Neopentane ··· Neopentane (D) | −77.1 | −103 | −103 | −90.8 | −96.2 | −71.8 | −97.2 | −91.8 |
| 37. | Cyclopentane ··· Neopentane (D) | −104 | −124 | −129 | −110 | −120 | −95.0 | −122 | −118 |
| 38. | Cyclopentane ··· Cyclopentane (D) | −130 | −147 | −152 | −131 | −147 | −118 | −145 | −143 |
| 39. | Benzene ··· Cyclopentane (D) | −155 | −158 | −176 | −150 | −153 | −135 | −157 | −163 |
| 40. | Benzene ··· Neopentane (D) | −126 | −135 | −146 | −128 | −126 | −109 | −131 | −134 |
| 41. | Uracil ··· Pentane (D) | −210 | −211 | −234 | −199 | −203 | −179 | −207 | −216 |
| 42. | Uracil ··· Cyclopentane (D) | −179 | −184 | −200 | −171 | −178 | −153 | −179 | −188 |
| 43. | Uracil ··· Neopentane (D) | −161 | −172 | −184 | −162 | −161 | −140 | −163 | −170 |
| 44. | Ethene ··· Pentane (D) | −86.9 | −100 | −96.5 | −89.3 | −96.9 | −75.5 | −90.5 | −87.4 |
| 45. | Ethyne ··· Pentane (D) | −75.8 | −94.9 | −91.4 | −85.3 | −89.4 | −71.2 | −82.3 | −82.3 |
| 46. | Peptide ··· Pentane (D) | −185 | −194 | −207 | −178 | −190 | −162 | −187 | −189 |
| | MD [meV] | — | −6.46 | −20.9 | 2.02 | −1.38 | 19.0 | −2.50 | −7.66 |
| | MAD [meV] | — | 13.0 | 20.9 | 7.71 | 10.6 | 19.0 | 7.84 | 8.06 |
| | MRD [%] | — | 8.11 | 15.6 | 0.77 | 4.22 | −11.7 | 4.08 | 6.13 |
| | MARD [%] | — | 10.4 | 15.6 | 5.12 | 7.82 | 11.7 | 6.21 | 6.39 |

TABLE S4. CONTINUED.

| No. | System (interaction type) | CCSD(T)/CBS | DF1 | DF1-optB88 | DF1-cx | DF2 | DF2-B86R | rVV10 | new |
|---|---|---|---|---|---|---|---|---|---|
| *Others (20)* | | | | | | | | | |
| 47. | Benzene ··· Benzene (TS) (D) | −125 | −118 | −126 | −114 | −111 | −100 | −115 | −119 |
| 48. | Pyridine ··· Pyridine (TS) (D) | −153 | −137 | −149 | −133 | −135 | −124 | −141 | −142 |
| 49. | Benzene ··· Pyridine (TS) (D) | −144 | −132 | −143 | −131 | −126 | −118 | −133 | −136 |
| 50. | Benzene ··· Ethyne (CH ··· $\pi$) (M) | −124 | −111 | −119 | −112 | −108 | −106 | −114 | −114 |
| 51. | Ethyne ··· Ethyne (TS) (M) | −66.1 | −67.7 | −66.1 | −64.2 | −70.0 | −63.0 | −72.9 | −65.4 |
| 52. | Benzene ··· AcOH (OH ··· $\pi$) (M) | −204 | −171 | −201 | −189 | −169 | −176 | −197 | −193 |
| 53. | Benzene ··· $AcNH_2$ (NH ··· $\pi$) (M) | −189 | −164 | −185 | −168 | −167 | −163 | −186 | −177 |
| 54. | Benzene ··· Water (OH ··· $\pi$) (M) | −142 | −121 | −136 | −126 | −125 | −124 | −141 | −131 |
| 55. | Benzene ··· MeOH (OH ··· $\pi$) (M) | −182 | −161 | −183 | −169 | −162 | −161 | −178 | −175 |
| 56. | Benzene ··· $MeNH_2$ (NH ··· $\pi$) (D) | −140 | −131 | −144 | −131 | −129 | −121 | −135 | −135 |
| 57. | Benzene ··· Peptide (NH ··· $\pi$) (M) | −229 | −206 | −232 | −212 | −199 | −196 | −216 | −220 |
| 58. | Pyridine ··· Pyridine (CH ··· N) (M) | −180 | −143 | −160 | −142 | −157 | −148 | −177 | −159 |
| 59. | Ethyne ··· Water (CH ··· O) (E) | −124 | −109 | −113 | −106 | −121 | −114 | −129 | −116 |
| 60. | Ethyne ··· AcOH (OH ··· $\pi$) (E) | −211 | −177 | −211 | −194 | −198 | −202 | −233 | −207 |
| 61. | Pentane ··· AcOH (D) | −126 | −143 | −147 | −131 | −136 | −112 | −131 | −133 |
| 62. | Pentane ··· $AcNH_2$ (D) | −153 | −161 | −170 | −147 | −159 | −134 | −160 | −157 |
| 63. | Benzene ··· AcOH(D) | −165 | −157 | −174 | −155 | −152 | −141 | −156 | −161 |
| 64. | Peptide ··· Ethene (M) | −130 | −129 | −133 | −120 | −131 | −113 | −129 | −125 |
| 65. | Pyridine ··· Ethyne (E) | −173 | −161 | −178 | −170 | −174 | −173 | −192 | −178 |
| 66. | $MeNH_2$ ··· Pyridine (M) | −172 | −158 | −178 | −158 | −168 | −157 | −176 | −170 |
| | MD [meV] | — | 13.7 | −0.83 | 13.1 | 11.8 | 19.3 | 0.98 | 6.08 |
| | MAD [meV] | — | 16.3 | 6.24 | 13.5 | 14.0 | 19.3 | 7.87 | 7.54 |
| | MRD [%] | — | −7.70 | 0.63 | −8.10 | −6.70 | −12.3 | −0.46 | −3.79 |
| | MARD [%] | — | 9.83 | 4.15 | 8.49 | 8.60 | 12.3 | 5.15 | 4.80 |
| *All complexes (66)* | | | | | | | | | |
| | MD [meV] | — | 19.8 | −8.05 | 9.75 | 10.0 | 14.9 | −9.29 | −0.99 |
| | MAD [meV] | — | 27.4 | 12.1 | 12.9 | 15.1 | 17.0 | 13.8 | 8.27 |
| | MRD [%] | — | −3.83 | 5.78 | −3.71 | −1.90 | −8.51 | 3.74 | 1.02 |
| | MARD [%] | — | 10.9 | 7.61 | 6.18 | 6.81 | 9.16 | 6.19 | 4.62 |

## IV. BINDING SEPARATION AND BINDING ENERGIES FOR THE X40 DATA SET

TABLE S5. Binding separations [Å] for the X40 set of molecular dimers. CCSD(T)/CBS reference values are from Ref. [5]. The interaction types are abbreviated as follows: disp = dispersion, ind = induction, $\mu$–$\mu$= dipole-dipole interaction, stack = stacking interaction, X = halogen bond, X–$\pi$= halogen–$\pi$ bond interaction, and HB = hydrogen bond.

| No. | Complex | Interaction/ halogen | CCSD(T)/ CBS | DF1 | DF1- optB88 | DF1-cx | DF2 | DF2- B86R | rVV10 | new |
|---|---|---|---|---|---|---|---|---|---|---|
| 1. | $CH_4 \cdots F_2$ | disp/F | 2.73 | 2.94 | 2.80 | 3.00 | 2.72 | 2.76 | 2.61 | 2.77 |
| 2. | $CH_4 \cdots Cl_2$ | disp/Cl | 3.13 | 3.55 | 3.34 | 3.59 | 3.36 | 3.34 | 3.21 | 3.36 |
| 3. | $CH_4 \cdots Br_2$ | disp/Br | 3.18 | 3.49 | 3.22 | 3.48 | 3.28 | 3.22 | 3.09 | 3.23 |
| 4. | $CH_4 \cdots I_2$ | disp/I | 3.38 | 3.71 | 3.42 | 3.67 | 3.50 | 3.43 | 3.28 | 3.44 |
| 5. | $CH_3F \cdots CH_4$ | ind/F | 2.83 | 3.21 | 3.12 | 3.28 | 3.04 | 3.13 | 3.00 | 3.14 |
| 6. | $CH_3Cl \cdots CH_4$ | ind/Cl | 2.79 | 3.20 | 3.07 | 3.26 | 3.03 | 3.09 | 2.97 | 3.10 |
| 7. | $CHF_3 \cdots CH_4$ | ind/F | 3.19 | 3.51 | 3.44 | 3.58 | 3.37 | 3.48 | 3.35 | 3.47 |
| 8. | $CHCl_3 \cdots CH_4$ | ind/Cl | 3.47 | 3.92 | 3.75 | 3.98 | 3.74 | 3.80 | 3.67 | 3.80 |
| 9. | $CH_3F \cdots CH_3F$ | $\mu$–$\mu$/F | 2.79 | 3.12 | 3.04 | 3.18 | 2.98 | 3.05 | 2.95 | 3.05 |
| 10. | $CH_3Cl \cdots CH_3Cl$ | $\mu$–$\mu$/Cl | 3.18 | 3.61 | 3.48 | 3.67 | 3.44 | 3.48 | 3.34 | 3.49 |
| 11. | $C_6H_3F_3 \cdots C_6H_6$ | stack/F | 3.29 | 3.56 | 3.33 | 3.40 | 3.46 | 3.37 | 3.35 | 3.36 |
| 12. | $C_6F_6 \cdots C_6H_6$ | stack/F | 3.32 | 3.55 | 3.35 | 3.39 | 3.46 | 3.38 | 3.37 | 3.37 |
| 13. | $CH_3Cl \cdots HCHO$ | X/Cl | 2.91 | 3.32 | 3.12 | 3.36 | 3.13 | 3.13 | 3.01 | 3.14 |
| 14. | $CH_3Br \cdots HCHO$ | X/Br | 3.12 | 3.36 | 3.13 | 3.29 | 3.18 | 3.14 | 3.04 | 3.14 |
| 15. | $CH_3I \cdots HCHO$ | X/I | 3.21 | 3.44 | 3.20 | 3.26 | 3.29 | 3.21 | 3.13 | 3.21 |
| 16. | $CF_3Cl \cdots HCHO$ | X/Cl | 2.98 | 3.31 | 3.13 | 3.24 | 3.16 | 3.13 | 3.07 | 3.14 |
| 17. | $CF_3Br \cdots HCHO$ | X/Br | 2.95 | 3.28 | 3.09 | 3.14 | 3.15 | 3.10 | 3.04 | 3.10 |
| 18. | $CF_3I \cdots HCHO$ | X/I | 3.01 | 3.31 | 3.13 | 3.15 | 3.22 | 3.14 | 3.10 | 3.14 |
| 19. | $C_6H_5Cl \cdots CH_3CHO$ | X/Cl | 3.12 | 3.49 | 3.30 | 3.48 | 3.33 | 3.33 | 3.23 | 3.32 |
| 20. | $C_6H_5Br \cdots CH_3CHO$ | X/Br | 3.06 | 3.29 | 3.07 | 3.16 | 3.14 | 3.09 | 3.01 | 3.08 |
| 21. | $C_6H_5I \cdots CH_3CHO$ | X/I | 3.09 | 3.28 | 3.06 | 3.09 | 3.17 | 3.07 | 3.01 | 3.07 |
| 22. | $C_6H_5Cl \cdots (CH_3)_3N$ | X/Cl | 3.06 | 3.19 | 2.98 | 3.01 | 3.09 | 2.99 | 2.97 | 2.99 |
| 23. | $C_6H_5Br \cdots (CH_3)_3N$ | X/Br | 2.97 | 3.12 | 2.92 | 2.92 | 3.05 | 2.92 | 2.92 | 2.92 |
| 24. | $C_6H_5I \cdots (CH_3)_3N$ | X/I | 2.97 | 3.12 | 2.94 | 2.92 | 3.09 | 2.94 | 2.94 | 2.94 |
| 25. | $C_6H_5Br \cdots CH_3SH$ | X/Br | 3.09 | 3.32 | 3.06 | 3.10 | 3.18 | 3.07 | 3.00 | 3.07 |
| 26. | $C_6H_5I \cdots CH_3SH$ | X/I | 3.35 | 3.54 | 3.29 | 3.27 | 3.44 | 3.29 | 3.26 | 3.29 |
| 27. | $CH_3Br \cdots C_6H_6$ | X–$\pi$/Br | 3.55 | 3.89 | 3.62 | 3.83 | 3.72 | 3.66 | 3.56 | 3.65 |
| 28. | $CH_3I \cdots C_6H_6$ | X–$\pi$/I | 3.66 | 4.01 | 3.72 | 3.82 | 3.85 | 3.75 | 3.65 | 3.74 |
| 29. | $CF_3Br \cdots C_6H_6$ | X–$\pi$/Br | 3.46 | 3.77 | 3.52 | 3.62 | 3.64 | 3.55 | 3.48 | 3.54 |
| 30. | $CF_3I \cdots C_6H_6$ | X–$\pi$/I | 3.53 | 3.84 | 3.56 | 3.59 | 3.72 | 3.59 | 3.53 | 3.58 |
| 31. | $CF_3OH \cdots H_2O$ | HB(OH–O)/F | 1.75 | 1.84 | 1.75 | 1.74 | 1.81 | 1.75 | 1.75 | 1.75 |
| 32. | $CCl_3OH \cdots H_2O$ | HB(OH–O)/Cl | 1.75 | 1.80 | 1.71 | 1.70 | 1.79 | 1.70 | 1.71 | 1.71 |
| 33. | $HF \cdots CH_3OH$ | HB(XH–O)/F | 1.69 | 1.75 | 1.68 | 1.67 | 1.73 | 1.68 | 1.67 | 1.68 |
| 34. | $HCl \cdots CH_3OH$ | HB(XH–O)/Cl | 1.85 | 1.96 | 1.83 | 1.81 | 1.92 | 1.81 | 1.81 | 1.82 |
| 35. | $HBr \cdots CH_3OH$ | HB(XH–O)/Br | 1.90 | 2.03 | 1.86 | 1.84 | 1.98 | 1.84 | 1.84 | 1.85 |
| 36. | $HI \cdots CH_3OH$ | HB(XH–O)/I | 2.03 | 2.21 | 1.99 | 1.97 | 2.12 | 1.97 | 1.95 | 1.97 |
| 37. | $HF \cdots CH_3NH_2$ | HB(XH–N)/F | 1.67 | 1.71 | 1.66 | 1.64 | 1.71 | 1.65 | 1.66 | 1.65 |
| 38. | $HCl \cdots CH_3NH_2$ | HB(XH–N)/Cl | 1.68 | 1.73 | 1.66 | 1.63 | 1.77 | 1.65 | 1.67 | 1.65 |
| 39. | $CH_3OH \cdots CH_3F$ | HB(OH–XC)/F | 1.99 | 2.25 | 2.12 | 2.18 | 2.15 | 2.12 | 2.08 | 2.12 |
| 40. | $CH_3OH \cdots CH_3Cl$ | HB(OH–XC)/Cl | 2.47 | 2.64 | 2.49 | 2.54 | 2.54 | 2.49 | 2.45 | 2.50 |
| | MD [Å] | | — | 0.25 | 0.07 | 0.16 | 0.13 | 0.08 | 0.02 | 0.08 |
| | MAD [Å] | | — | 0.25 | 0.09 | 0.19 | 0.13 | 0.11 | 0.08 | 0.10 |
| | MRD [%] | | — | 8.55 | 2.25 | 5.03 | 4.63 | 2.48 | 0.41 | 2.51 |
| | MARD [%] | | — | 8.55 | 3.22 | 6.27 | 4.64 | 3.62 | 2.66 | 3.59 |

TABLE S6. Binding energies [meV] for the X40 set of molecular dimers. CCSD(T)/CBS reference values are from Ref. [5]. The interaction types are abbreviated as follows: disp = dispersion, ind = induction, $\mu$–$\mu$= dipole-dipole interaction, stack = stacking interaction, X = halogen bond, X–$\pi$= halogen–$\pi$ bond interaction, and HB = hydrogen bond. The outliers in Fig. 6 in the main manuscript are indicated in red.

| No. | Complex | Interaction/ halogen | CCSD(T)/ CBS | DF1 | DF1 optB88 | DF1-cx | DF2 | DF2 -B86R | rVV10 | new |
|---|---|---|---|---|---|---|---|---|---|---|
| 1. | $CH_4 \cdots F_2$ | disp/F | −21.3 | −36.8 | −26.0 | −31.0 | −40.4 | −27.9 | −40.6 | −30.3 |
| 2. | $CH_4 \cdots Cl_2$ | disp/Cl | −46.8 | −49.5 | −44.2 | −44.0 | −51.6 | −41.6 | −53.2 | −44.2 |
| 3. | $CH_4 \cdots Br_2$ | disp/Br | −56.4 | −53.6 | −52.6 | −48.4 | −57.6 | −49.0 | −66.2 | −51.9 |
| 4. | $CH_4 \cdots I_2$ | disp/I | −58.4 | −54.6 | −54.4 | −49.7 | −57.7 | −49.6 | −69.8 | −53.4 |
| 5. | $CH_3F \cdots CH_4$ | ind/F | −32.6 | −47.1 | −33.8 | −41.0 | −41.1 | −28.8 | −31.8 | −32.3 |
| 6. | $CH_3Cl \cdots CH_4$ | ind/Cl | −42.5 | −54.4 | −43.0 | −47.9 | −49.4 | −36.1 | −40.2 | −40.2 |
| 7. | $CHF_3 \cdots CH_4$ | ind/F | −30.0 | −53.0 | −38.1 | −46.2 | −42.2 | −28.6 | −33.5 | −35.3 |
| 8. | $CHCl_3 \cdots CH_4$ | ind/Cl | −49.7 | −68.2 | −58.0 | −60.2 | −60.2 | −43.9 | −52.6 | −52.2 |
| 9. | $CH_3F \cdots CH_3F$ | $\mu$–$\mu$/F | −71.5 | −76.0 | −63.0 | −67.2 | −76.1 | −59.4 | −64.9 | −63.1 |
| 10. | $CH_3Cl \cdots CH_3Cl$ | $\mu$–$\mu$/Cl | −58.0 | −59.6 | −49.9 | −53.6 | −57.0 | −45.4 | −51.5 | −49.5 |
| 11. | $C_6H_3F_3 \cdots C_6H_6$ | stack/F | −191 | −198 | −225 | −197 | −185 | −169 | −190 | −208 |
| 12. | $C_6F_6 \cdots C_6H_6$ | stack/F | −265 | −271 | −308 | −278 | −255 | −241 | −263 | −290 |
| 13. | $CH_3Cl \cdots HCHO$ | X/Cl | −50.7 | −53.3 | −48.3 | −45.3 | −60.1 | −44.9 | −61.5 | −49.1 |
| 14. | $CH_3Br \cdots HCHO$ | X/Br | −74.7 | −68.4 | −71.4 | −60.3 | −82.0 | −67.0 | −93.0 | −71.7 |
| 15. | $CH_3I \cdots HCHO$ | X/I | −103 | −90.0 | −103 | −88.2 | −109 | −97.5 | −131 | −103 |
| 16. | $CF_3Cl \cdots HCHO$ | X/Cl | −97.4 | −90.4 | −95.5 | −82.5 | −107 | −89.5 | −110 | −94.3 |
| 17. | $CF_3Br \cdots HCHO$ | X/Br | −135 | −116 | −131 | −113 | −140 | −124 | −153 | −129 |
| 18. | $CF_3I \cdots HCHO$ | X/I | −177 | −149 | −176 | −157 | −178 | −168 | −204 | −174 |
| 19. | $C_6H_5Cl \cdots CH_3CHO$ | X/Cl | −64.6 | −69.8 | −70.2 | −61.8 | −73.3 | −56.8 | −77.7 | −66.7 |
| 20. | $C_6H_5Br \cdots CH_3CHO$ | X/Br | −105 | −96.8 | −109 | −91.8 | −110 | −94.0 | −126 | −105 |
| 21. | $C_6H_5I \cdots CH_3CHO$ | X/I | −150 | −132 | −158 | −138 | −152 | −142 | −183 | −153 |
| 22. | $C_6H_5Cl \cdots (CH_3)_3N$ | X/Cl | −91.6 | −105 | −123 | −111 | −110 | −103 | −122 | −117 |
| 23. | $C_6H_5Br \cdots (CH_3)_3N$ | X/Br | −164 | −154 | −194 | −181 | −169 | −174 | −201 | −188 |
| 24. | $C_6H_5I \cdots (CH_3)_3N$ | X/I | −252 | −220 | −287 | −277 | −240 | −266 | −299 | −282 |
| 25. | $C_6H_5Br \cdots CH_3SH$ | X/Br | −100 | −88.4 | −105 | −89.9 | −102 | −93.7 | −125 | −102 |
| 26. | $C_6H_5I \cdots CH_3SH$ | X/I | −134 | −113 | −148 | −135 | −133 | −136 | −176 | −144 |
| 27. | $CH_3Br \cdots C_6H_6$ | X–$\pi$/Br | −78.7 | −80.5 | −84.3 | −73.3 | −79.4 | −64.8 | −84.8 | −78.0 |
| 28. | $CH_3I \cdots C_6H_6$ | X–$\pi$/I | −108 | −98.7 | −112 | −95.2 | −100 | −89.3 | −117 | −104 |
| 29. | $CF_3Br \cdots C_6H_6$ | X–$\pi$/Br | −135 | −117 | −132 | −115 | −120 | −109 | −133 | −124 |
| 30. | $CF_3I \cdots C_6H_6$ | X–$\pi$/I | −170 | −138 | −166 | −145 | −145 | −140 | −172 | −156 |
| 31. | $CF_3OH \cdots H_2O$ | HB(OH–O)/F | −419 | −364 | −417 | −403 | −398 | −413 | −443 | −417 |
| 32. | $CCl_3OH \cdots H_2O$ | HB(OH–O)/Cl | −451 | −389 | −462 | −449 | −423 | −457 | −489 | −462 |
| 33. | $HF \cdots CH_3OH$ | HB(XH–O)/F | −416 | −361 | −413 | −397 | −405 | −415 | −446 | −416 |
| 34. | $HCl \cdots CH_3OH$ | HB(XH–O)/Cl | −273 | −225 | −269 | −260 | −251 | −271 | −292 | −273 |
| 35. | $HBr \cdots CH_3OH$ | HB(XH–O)/Br | −232 | −188 | −233 | −227 | −211 | −235 | −255 | −238 |
| 36. | $HI \cdots CH_3OH$ | HB(XH–O)/I | −172 | −136 | −170 | −164 | −153 | −171 | −193 | −175 |
| 37. | $HF \cdots CH_3NH_2$ | HB(XH–N)/F | −621 | −578 | −656 | −653 | −614 | −661 | −692 | −661 |
| 38. | $HCl \cdots CH_3NH_2$ | HB(XH–N)/Cl | −495 | −451 | −548 | −566 | −461 | −559 | −568 | −559 |
| 39. | $CH_3OH \cdots CH_3F$ | HB(OH–XC)/F | −169 | −147 | −158 | −143 | −167 | −152 | −172 | −157 |
| 40. | $CH_3OH \cdots CH_3Cl$ | HB(OH–XC)/Cl | −164 | −144 | −159 | −145 | −161 | −152 | −173 | −157 |
| | MD [meV] | | — | 13.5 | −6.74 | 2.41 | 2.47 | 3.99 | −18.1 | −4.53 |
| | MAD [meV] | | — | 19.9 | 10.4 | 14.1 | 9.86 | 11.9 | 19.2 | 9.46 |
| | MRD [%] | | — | −0.12 | 3.93 | −0.95 | 5.11 | −5.93 | 13.4 | 1.86 |
| | MARD [%] | | — | 15.6 | 7.79 | 12.4 | 10.2 | 9.90 | 15.0 | 7.06 |

## V. LATTICE CONSTANTS AND ATOMIZATION ENERGIES FOR SELECTED SOLIDS

TABLE S7. Lattice constants [Å] for a list of 23 selected solids, assembled by Klimes et al.[6] The reference data are based on zero-point corrected experimental lattice constants and atomization energies, as detailed in Ref. [6] and references therein. The outliers in Fig. 7 in the main manuscript are indicated in red.

| Solids | Experiment | vdW-DF1 | vdW-DF1-optB88 | vdW-DF1-cx | vdW-DF2 | vdW-DF2-B86R | rVV10 | new |
|---|---|---|---|---|---|---|---|---|
| Cu | 3.60 | 3.69 | 3.62 | 3.57 | 3.75 | 3.59 | 3.65 | 3.59 |
| Ag | 4.06 | 4.25 | 4.14 | 4.07 | 4.33 | 4.11 | 4.17 | 4.10 |
| Pd | 3.88 | 4.01 | 3.94 | 3.89 | 4.09 | 3.92 | 3.98 | 3.91 |
| Rh | 3.79 | 3.88 | 3.84 | 3.79 | 3.95 | 3.81 | 3.87 | 3.81 |
| Li | 3.45 | 3.44 | 3.42 | 3.49 | 3.39 | 3.43 | 3.41 | 3.43 |
| Na | 4.21 | 4.21 | 4.15 | 4.24 | 4.14 | 4.17 | 4.13 | 4.16 |
| K | 5.21 | 5.31 | 5.21 | 5.32 | 5.20 | 5.24 | 5.14 | 5.22 |
| Rb | 5.58 | 5.60 | 5.49 | 5.59 | 5.51 | 5.53 | 5.46 | 5.52 |
| Cs | 6.04 | 6.00 | 5.83 | 5.90 | 5.93 | 5.89 | 5.84 | 5.86 |
| Ca | 5.55 | 5.54 | 5.44 | 5.46 | 5.48 | 5.46 | 5.46 | 5.45 |
| Sr | 6.04 | 6.07 | 5.92 | 5.93 | 6.02 | 5.94 | 5.93 | 5.93 |
| Ba | 5.00 | 5.07 | 4.91 | 4.87 | 5.05 | 4.92 | 4.92 | 4.90 |
| Al | 4.02 | 4.09 | 4.06 | 4.03 | 4.09 | 4.04 | 4.03 | 4.04 |
| LiF | 3.96 | 4.11 | 4.03 | 4.06 | 4.08 | 4.04 | 4.03 | 4.04 |
| LiCl | 5.06 | 5.22 | 5.12 | 5.11 | 5.21 | 5.11 | 5.11 | 5.10 |
| NaF | 4.58 | 4.76 | 4.66 | 4.71 | 4.70 | 4.67 | 4.65 | 4.67 |
| NaCl | 5.57 | 5.75 | 5.63 | 5.67 | 5.70 | 5.64 | 5.61 | 5.63 |
| MgO | 4.18 | 4.28 | 4.23 | 4.23 | 4.29 | 4.23 | 4.25 | 4.23 |
| C | 3.54 | 3.59 | 3.58 | 3.57 | 3.61 | 3.57 | 3.59 | 3.57 |
| SiC | 4.34 | 4.40 | 4.38 | 4.37 | 4.43 | 4.38 | 4.40 | 4.38 |
| Si | 5.42 | 5.51 | 5.48 | 5.44 | 5.55 | 5.46 | 5.50 | 5.46 |
| Ge | 5.64 | 5.84 | 5.73 | 5.67 | 5.94 | 5.71 | 5.80 | 5.70 |
| GaAs | 5.64 | 5.84 | 5.74 | 5.68 | 5.93 | 5.72 | 5.79 | 5.71 |
| MD [Å] | — | 0.09 | 0.01 | 0.01 | 0.09 | 0.01 | 0.02 | 0.002 |
| MAD [Å] | — | 0.10 | 0.07 | 0.06 | 0.12 | 0.06 | 0.09 | 0.06 |
| MRD [%] | — | 2.01 | 0.29 | 0.35 | 1.99 | 0.28 | 0.49 | 0.12 |
| MARD [%] | — | 2.12 | 1.43 | 1.13 | 2.71 | 1.14 | 1.77 | 1.15 |

TABLE S8. Atomization energies [eV] for a list of 23 selected solids, assembled by Klimes et al.[6] The reference data are based on zero-point corrected experimental lattice constants and atomization energies, as detailed in Ref. [6] and references therein. The outliers in Fig. 7 in the main manuscript are indicated in red.

| Solids | Experiment | vdW-DF1 | vdW-DF1-optB88 | vdW-DF1-cx | vdW-DF2 | vdW-DF2-B86R | rVV10 | new |
|---|---|---|---|---|---|---|---|---|
| Cu | 3.52 | 3.07 | 3.59 | 3.90 | 2.89 | 3.70 | 3.72 | 3.80 |
| Ag | 2.98 | 2.29 | 2.76 | 2.98 | 2.15 | 2.79 | 2.89 | 2.90 |
| Pd | 3.94 | 3.36 | 4.00 | 4.32 | 3.16 | 4.09 | 4.13 | 4.21 |
| Rh | 5.78 | 4.99 | 6.06 | 6.72 | 4.69 | 6.26 | 5.92 | 6.52 |
| Li | 1.67 | 1.46 | 1.52 | 1.59 | 1.43 | 1.56 | 1.59 | 1.56 |
| Na | 1.12 | 0.96 | 0.99 | 1.20 | 0.96 | 1.01 | 1.07 | 1.03 |
| K | 0.94 | 0.82 | 0.85 | 0.90 | 0.73 | 0.84 | 0.94 | 0.86 |
| Rb | 0.86 | 0.77 | 0.78 | 0.81 | 0.66 | 0.76 | 0.87 | 0.79 |
| Cs | 0.81 | 0.79 | 0.76 | 0.77 | 0.64 | 0.72 | 0.87 | 0.76 |
| Ca | 1.86 | 1.66 | 1.86 | 2.04 | 1.40 | 1.87 | 2.00 | 1.91 |
| Sr | 1.73 | 1.42 | 1.61 | 1.78 | 1.12 | 1.60 | 1.73 | 1.65 |
| Ba | 1.91 | 1.79 | 1.99 | 2.14 | 1.49 | 1.95 | 2.10 | 2.01 |
| Al | 3.43 | 2.90 | 3.24 | 3.64 | 2.52 | 3.43 | 3.41 | 3.44 |
| LiF | 4.46 | 4.44 | 4.56 | 4.44 | 4.57 | 4.49 | 4.55 | 4.51 |
| LiCl | 3.59 | 3.42 | 3.54 | 3.51 | 3.44 | 3.49 | 3.53 | 3.52 |
| NaF | 3.98 | 3.97 | 4.04 | 4.02 | 4.08 | 3.97 | 4.03 | 3.99 |
| NaCl | 3.34 | 3.18 | 3.26 | 3.29 | 3.19 | 3.19 | 3.24 | 3.22 |
| MgO | 5.20 | 4.95 | 5.06 | 5.27 | 4.93 | 5.20 | 5.26 | 5.23 |
| C | 7.55 | 7.13 | 7.60 | 7.89 | 6.87 | 7.76 | 7.61 | 7.77 |
| SiC | 6.48 | 5.95 | 6.38 | 6.61 | 5.72 | 6.48 | 6.34 | 6.50 |
| Si | 4.68 | 4.19 | 4.55 | 4.75 | 4.00 | 4.62 | 4.57 | 4.64 |
| Ge | 3.92 | 3.30 | 3.82 | 3.98 | 3.31 | 3.84 | 3.86 | 3.91 |
| GaAs | 3.34 | 2.85 | 3.27 | 3.40 | 2.80 | 3.27 | 3.35 | 3.33 |
| MD [eV] | — | −0.32 | −0.04 | 0.12 | −0.45 | −0.01 | 0.02 | 0.04 |
| MAD [eV] | — | 0.32 | 0.10 | 0.16 | 0.47 | 0.10 | 0.08 | 0.11 |
| MRD [%] | — | −10.3 | −2.81 | 2.82 | −15.8 | −2.33 | 0.93 | −0.52 |
| MARD [%] | — | 10.3 | 4.31 | 4.87 | 16.2 | 4.35 | 2.99 | 4.08 |

* Email: kristian.berland@nmbu.no
† E-mail: thonhauser@wfu.edu


[1] E. Schröder, V. R. Cooper, K. Berland, B. I. Lundqvist, P. Hyldgaard, and T. Thonhauser, in *Non-Covalent Interact. Quantum Chem. Phys. Theory Appl.*, edited by A. O. de la Roza and G. A. DiLabio (Elsevier, Amsterdam, 2017) Chap. 8, pp. 241–274.
[2] M. Dion, H. Rydberg, E. Schröder, D. C. Langreth, and B. I. Lundqvist, Phys. Rev. Lett. **92**, 246401 (2004).
[3] T. Takatani, E. G. Hohenstein, M. Malagoli, M. S. Marshall, and C. D. Sherrill, J. Chem. Phys. **132**, 144104 (2010).
[4] J. Řezáč, K. E. Riley, and P. Hobza, J. Chem. Theory Comput. **7**, 2427 (2011).
[5] J. Řezáč, K. E. Riley, and P. Hobza, J. Chem. Theory Comput. **8**, 4285 (2012).
[6] J. Klimeš, D. R. Bowler, and A. Michaelides, Phys. Rev. B **83**, 195131 (2011).
